# Supplementary material for: PatchNet: Hierarchical Deep Learning-Based Stable Patch Identification for the Linux Kernel
Source: arXiv:1911.03576 source file (2019-11-08)
Supplement: Supplementary file 1 [file appendix2.tex]

% \appendix
% \section{Some examples}

% \jg{JULIA--Please recheck this paragraph} 
% To illustrate the effect of our approach, we provide a few mainline Linux kernel commit ids from our results.  Examples of true
% positives not found by the other baselines ({\em cf.}
% Figure \ref{fig:venn_diagram}) include 5567e989198b and 2e31b4cb895a.
% Examples of false negatives found by at least one other baseline include
% 03f219041fdb and 56199016e867.  Most of PatchNet's top 100 false positives
% appear to the authors to be stable-relevant patches that have been
% overlooked by kernel maintainers.  Examples include e2bd416f6246 and
% acf2dc2266b9.
